# Supplementary material for: Few-shot Medical Image Segmentation with Cycle-resemblance Attention
Source: arXiv:2212.03967 source file (2022-12-07)
Supplement: Supplementary file 1 [file 6_Supplementary_Materials.tex]

\section*{Supplementary Material}

\noindent\textbf{Qualitative Results of Experiments in \textit{setting 2}.} 
In order to further demonstrate the visual segmentation results of both settings, we also show some qualitative results under \textbf{\textit{setting 2}} on both datasets in Figures.~\ref{suppct} and~\ref{suppmri}.
As can be seen, for the abdominal CT dataset, our proposed method makes a segmentation that covers most of the \textit{liver} area, while the result of SSL-ALPNet only covers half of the \textit{liver}.
Moreover, the segmentation results of SSL-APLNet have visible false positive volumes for the examples in \textit{left kidney}, \textit{right kidney} and \textit{spleen}, while our method makes segmentation which are closed to the ground truth for those 
\begin{figure}[H]
\centering
\includegraphics[width=1\linewidth]{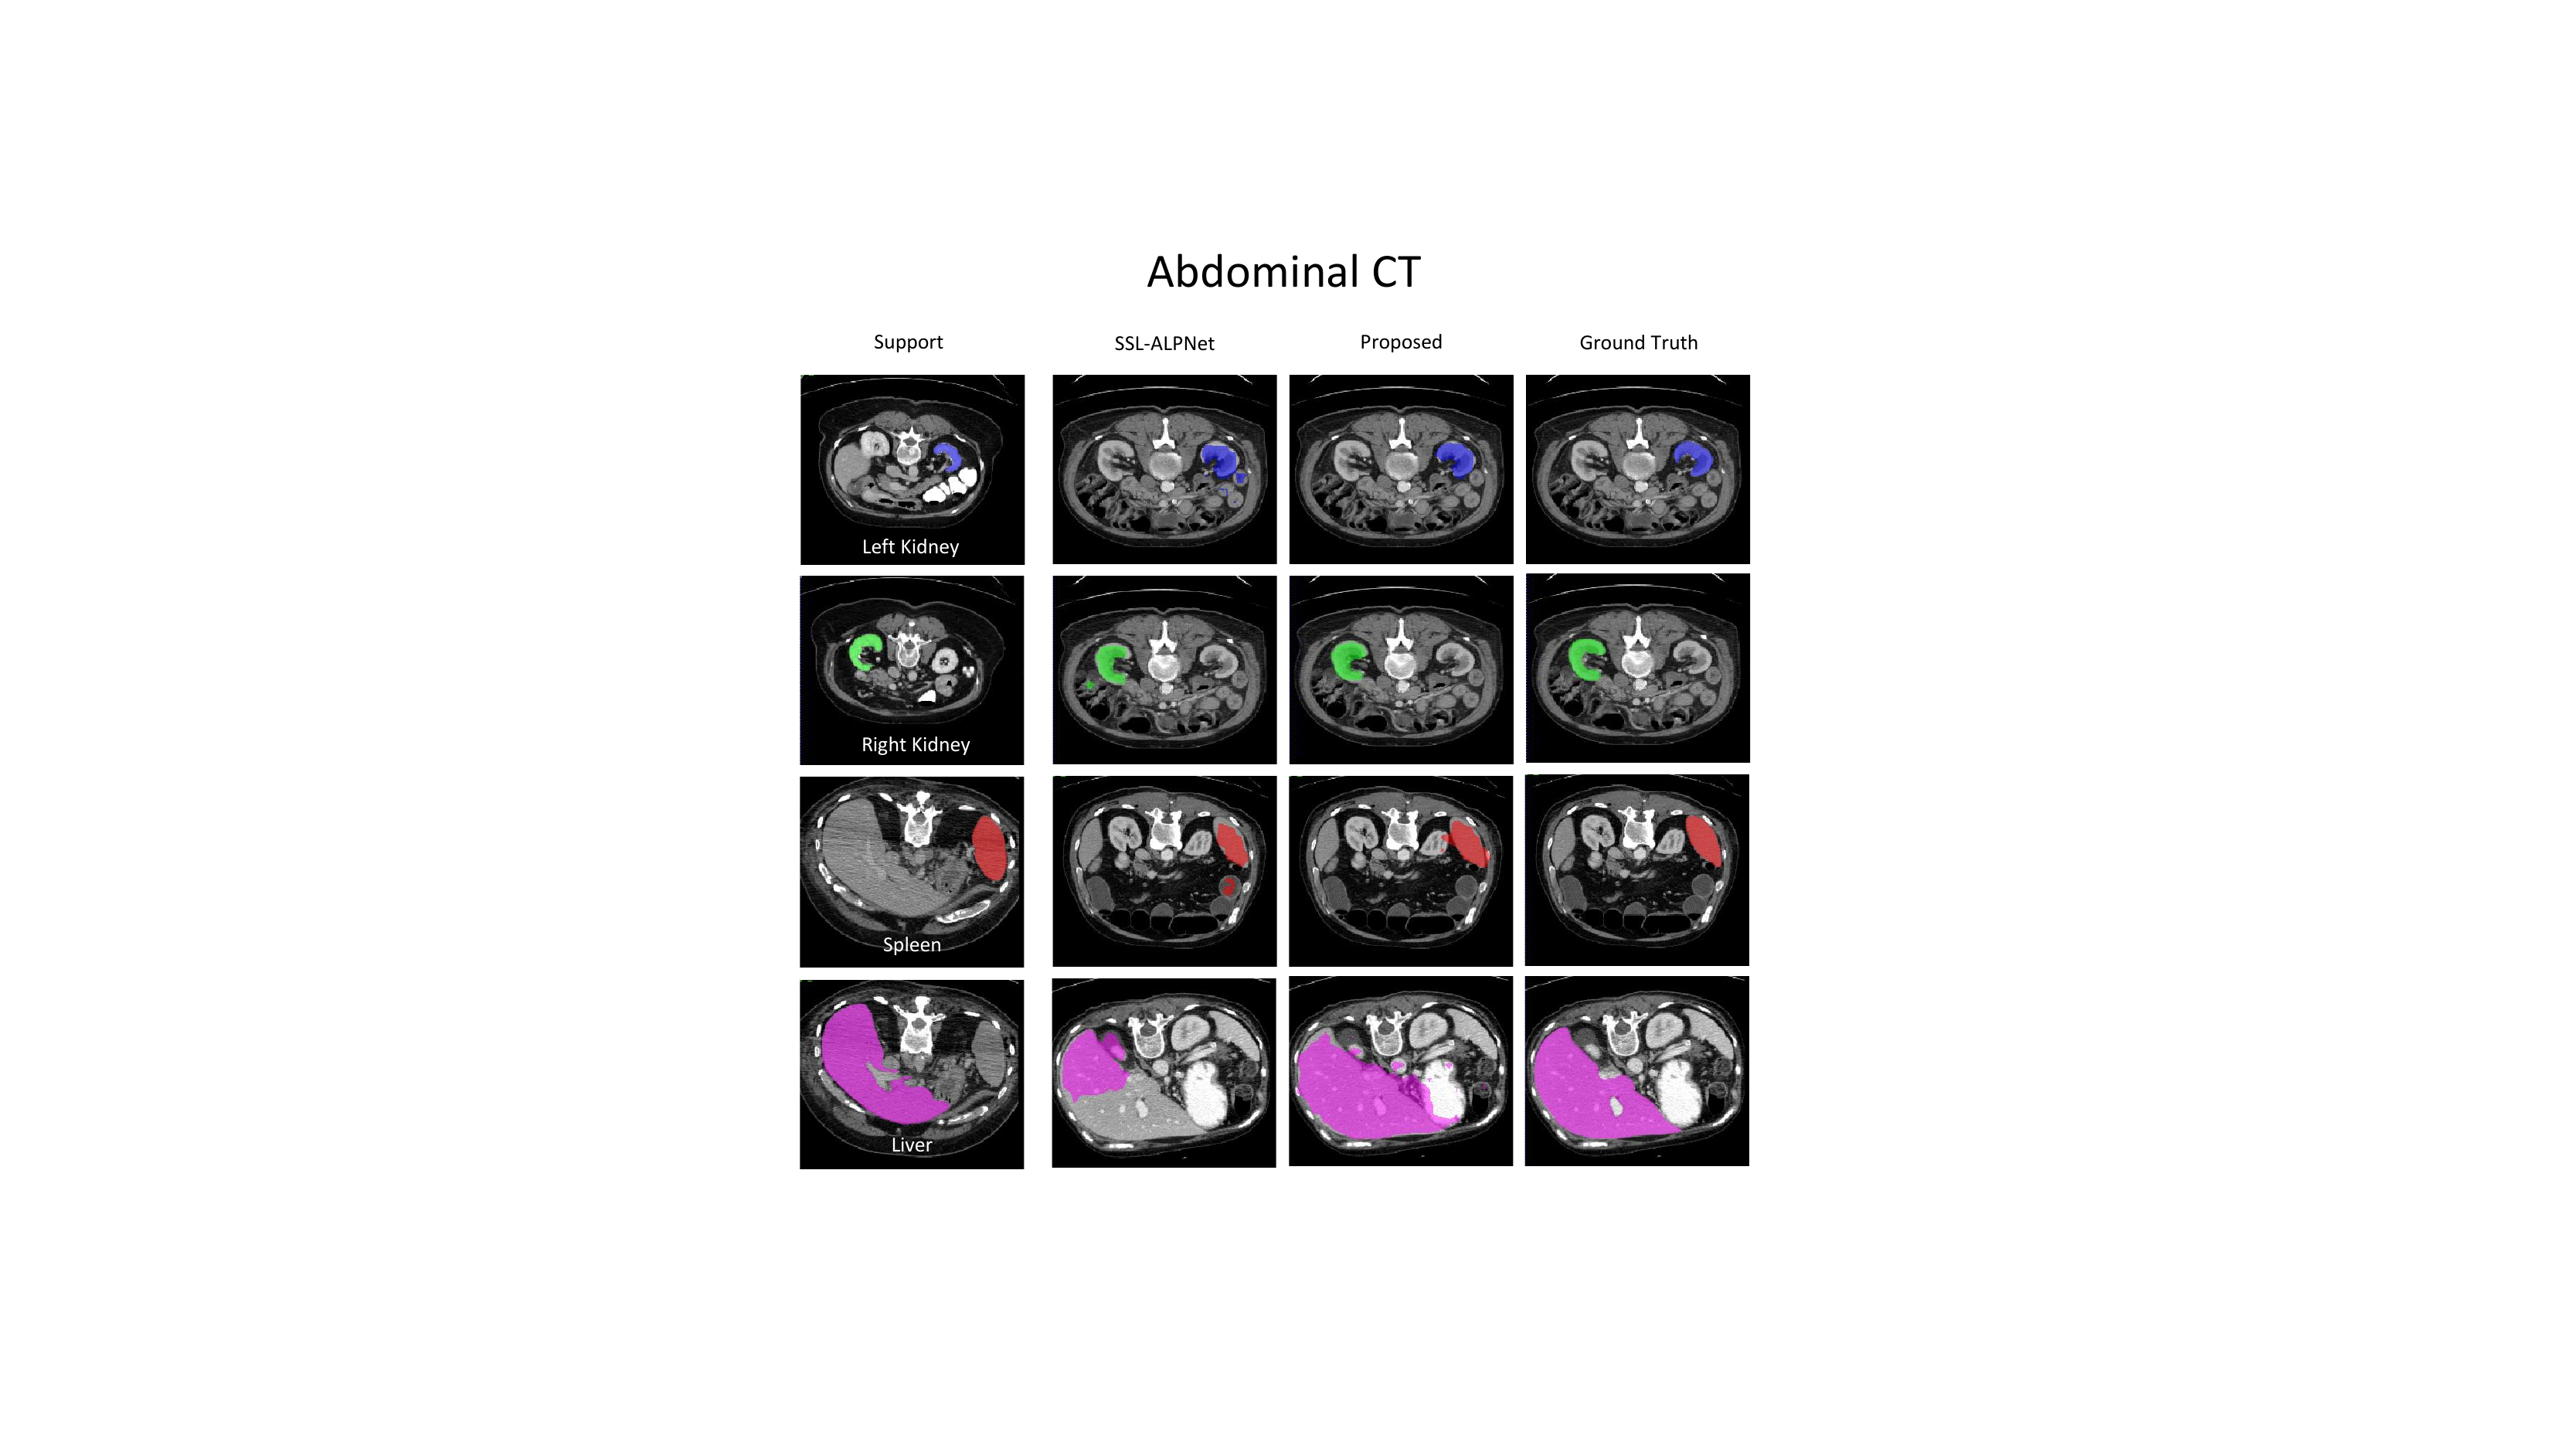}
   \caption{The qualitative results under \textbf{\textit{setting 2}} on abdominal-CT dataset.}
\label{suppct}
\end{figure}
\noindent classes. For the abdominal MRI dataset, our method performs a better segmentation of the class \textit{spleen} and \textit{liver} than that of the SSL-ALPNet. 
Last, our segmentation result of \textit{left kidney} and \textit{right kidney} aligns closer to the ground truth class boundary than results of SSL-ALPNet does.
Therefore, our approach makes a more precise segmentation especially on drawing the boundary of the classes.

\begin{figure}[t]
\centering
\includegraphics[width=1\linewidth]{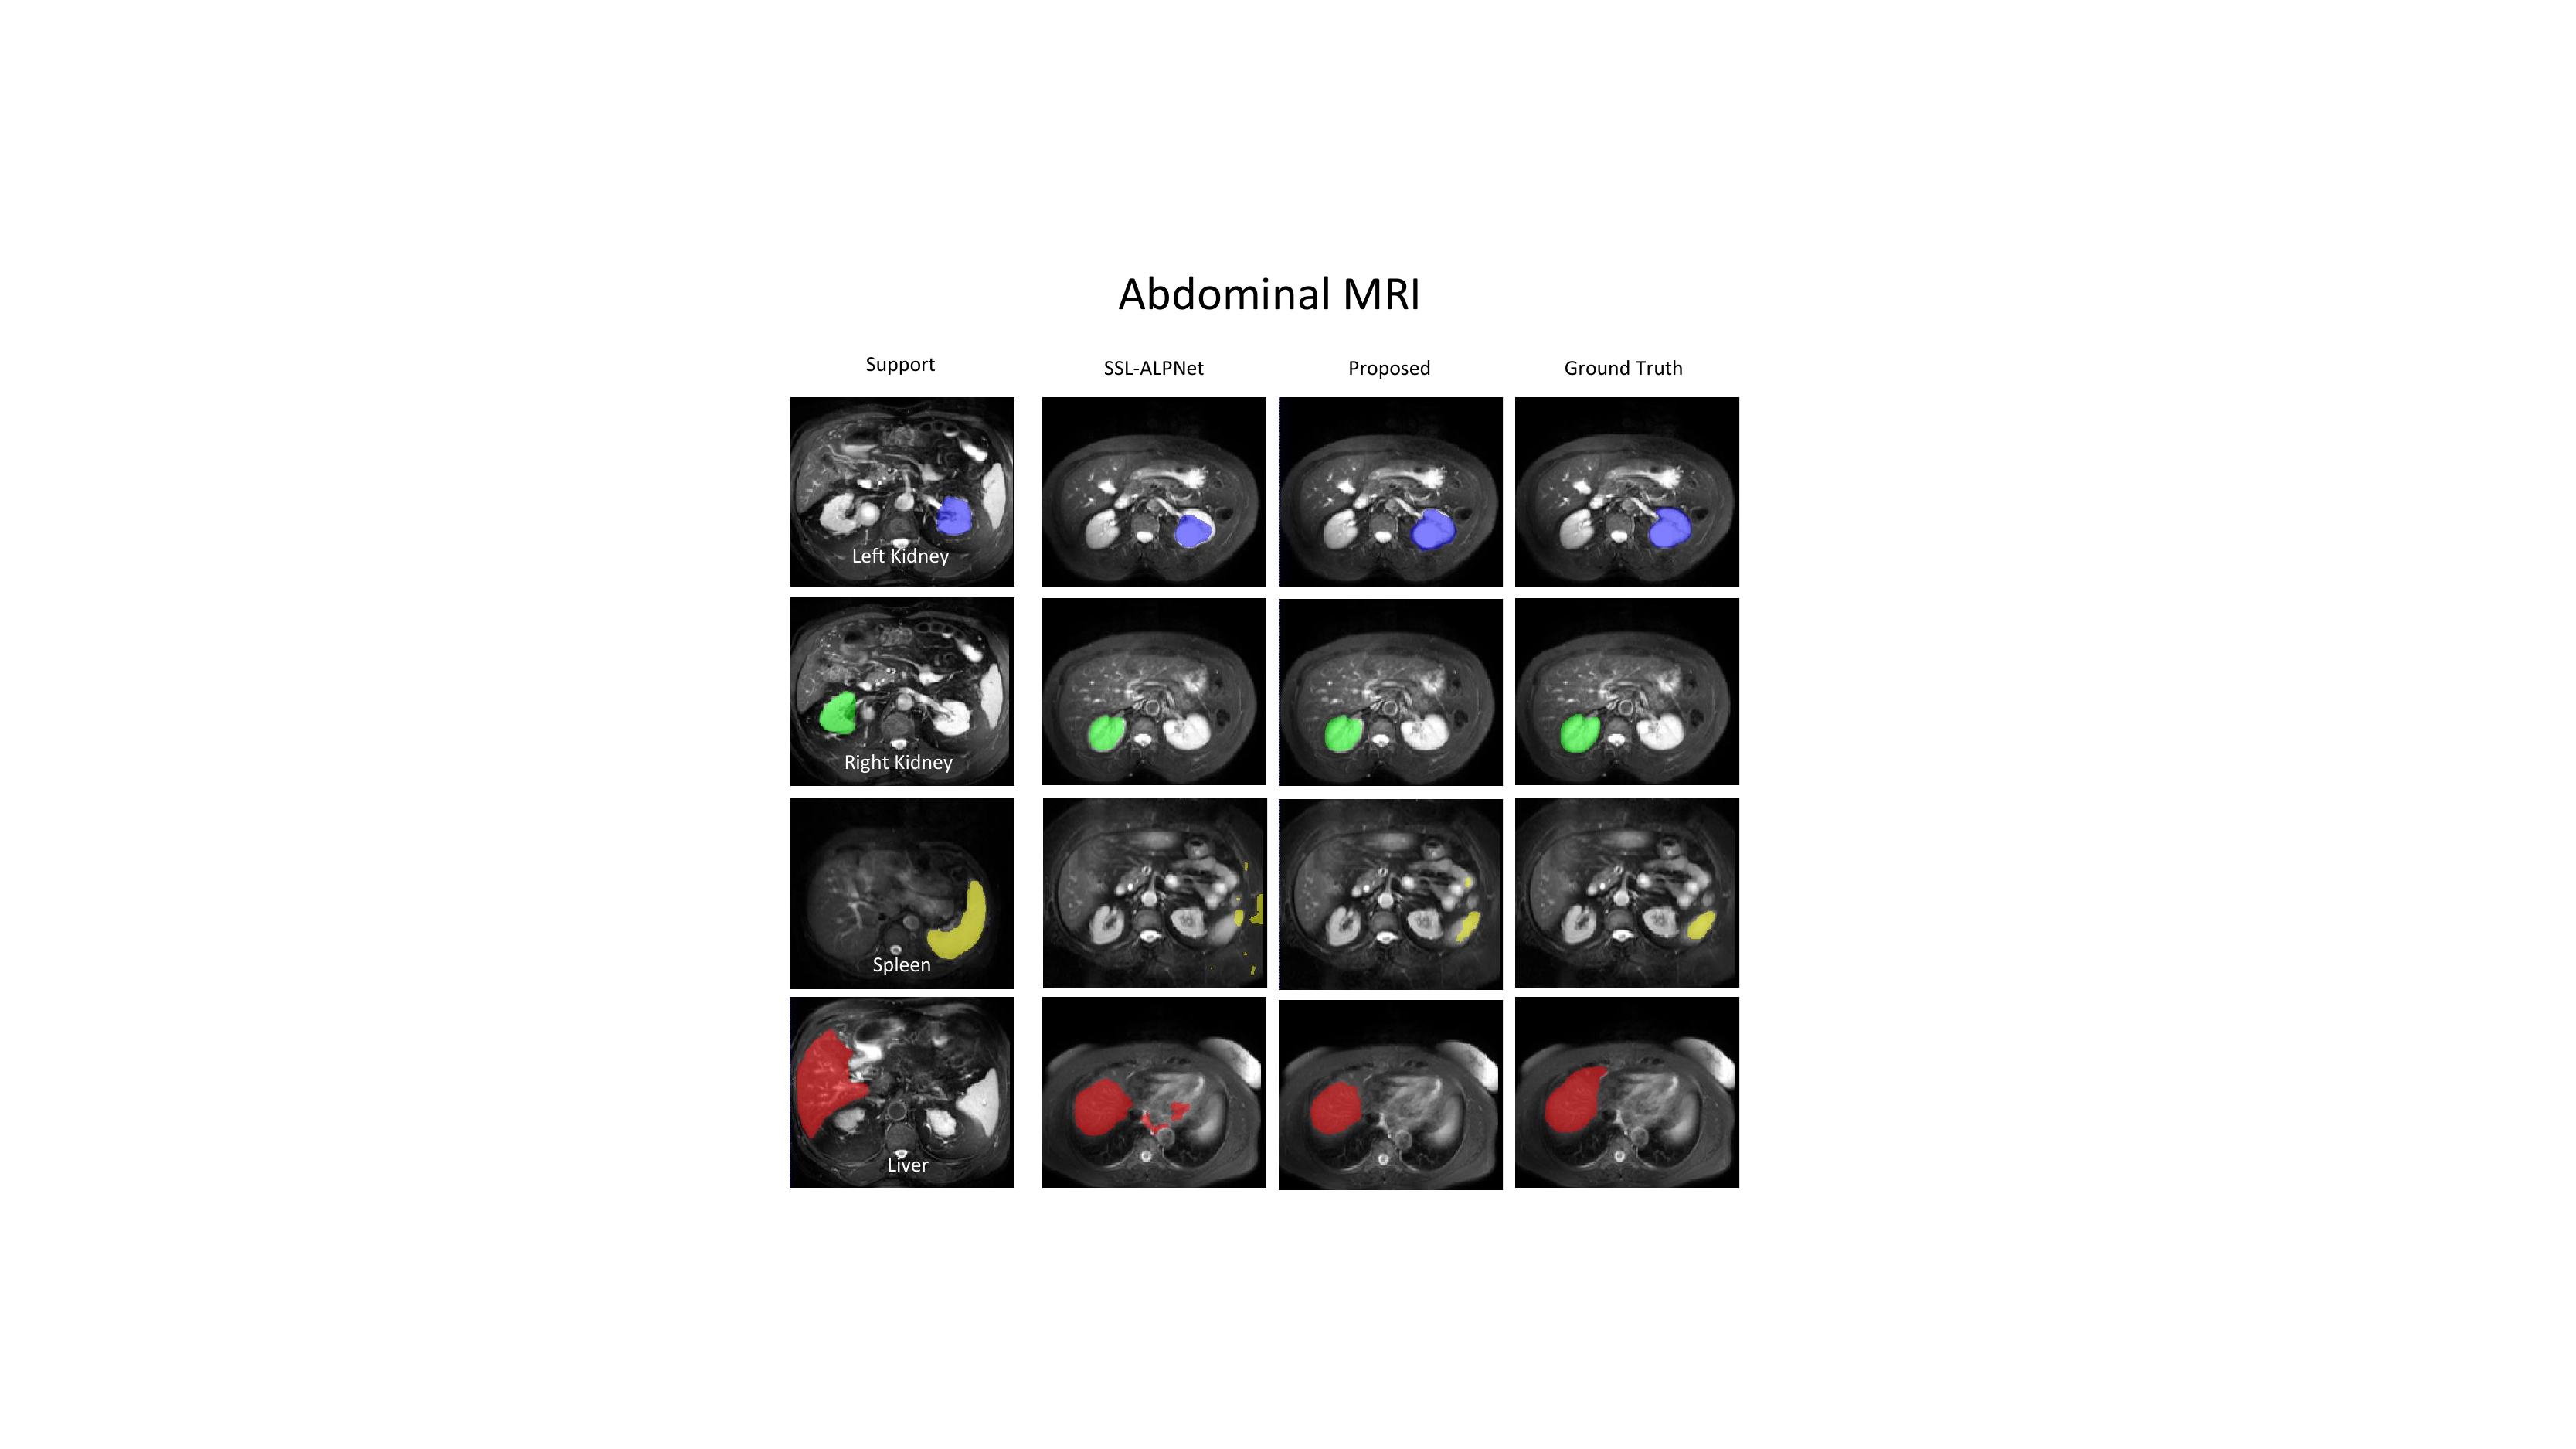}
   \caption{The qualitative results under \textbf{\textit{setting 2}} on abdominal-MRI dataset.}
\label{suppmri}
\end{figure}

\begin{table}[H]
\centering
\begin{tabular}{cccccc}
\toprule
\# of Blocks     & LK             & RK             & Spleen         & Liver          & Mean           \\ \midrule
1                & 80.39          & 82.42          & \textbf{74.52} & 71.93          & 77.30          \\
3                & \textbf{82.45} & 85.06          & 72.16          & 75.94          & 78.90          \\
5                & 81.95          & \textbf{86.42} & \textbf{74.32} & \textbf{76.46} & \textbf{79.79} \\
7                & 82.08          & 83.93          & 73.35          & 73.16          & 78.13          \\
9                & 80.27          & 83.93          & 73.61          & 74.28          & 78.02          \\
12               & 82.41          & 85.84          & 71.88          & 73.02          & 78.29          \\
15               & 80.71          & 86.00          & 73.88          & 72.67          & 78.31          \\ \bottomrule
\end{tabular}
\caption{Experiments results (in Dice Score) on the number of Cyc-Resemblance blocks on abdominal MRI in \textit{\textbf{setting~1}}.}
\label{supblocks}
\end{table}

\begin{algorithm*}[h] \small
    \PyFunc{def} \PyCode{ \textsc{cra}(sup\_ft, qry\_ft, num\_block):} \PyComment{Cycle-Resemblance Attention Module}\\
    \PyCode{~~~~init\_sup\_ft = sup\_ft.detach().clone()} \PyComment{copy initial support feature}\\
    \PyCode{~~~~init\_qry\_ft = qry\_ft.detach().clone()} \PyComment{copy initial query feature}\\
    \PyCode{~~~~for n in range(num\_block):}\\
    \PyCode{~~~~~~~~sup\_ft = \textsc{update\_ft}(sup\_ft, init\_qry\_ft)} \PyComment{Update the support feature}\\
    \PyCode{~~~~~~~~qry\_ft = \textsc{update\_ft}(qry\_ft, init\_sup\_ft)} \PyComment{Update the query feature}\\
    \PyFunc{~~~~return} \PyCode{sup\_ft, qry\_ft} \\
    
    \PyFunc{def} \PyCode{\textsc{update\_ft}(ft\_A, ft\_B):} \PyComment{Returns the updated feature A}\\
    \PyCode{~~~~g\_ft\_A = g(ft\_A)} \PyComment{g is a $1\times 1\times 1$ torch.nn.Conv2d layer}\\
    \PyCode{~~~~phi\_ft\_A = phi(ft\_A)} \PyComment{phi is a $1\times 1\times 1$ torch.nn.Conv2d layer}\\
    \PyCode{~~~~theta\_ft\_B = theta(ft\_B)} \PyComment{theta is a $1\times 1\times 1$ torch.nn.Conv2d layer}\\
    \PyCode{~~~~ftA\_flat = torch.flatten(ft\_A)} \PyComment{flatten the feature tensor}\\
    \PyCode{~~~~ftB\_flat = torch.flatten(ft\_B)} \\
    \PyCode{~~~~affine = ftA\_flat @ ftB\_flat.transpose()} \PyComment{Matrix mult.; A as row, B as col}\\ 
    \PyCode{~~~~ftA2ftB\_idx = affine.max(dim=column)[1]} \PyComment{col index with max value for each row}\\
    \PyCode{~~~~ftB2ftA\_star\_idx = affine.max(dim=row)[1]} \\
    
    \PyCode{~~~~}\PyComment{find the most resemble pixel $i^*$ of pixel $i$ in feature A }\\
    \PyCode{~~~~}\PyComment{via cycle resemblance operation}\\
    \PyCode{~~~~ftA2ftA\_star\_idx = torch.gather(ftA2ftB\_idx, ftB2ftA\_idx)} \\
    \PyCode{~~~~ftA\_star\_flat = torch.gather(ftA\_flat, ftA2ftA\_star\_idx)} \\
    
    \PyCode{~~~~}\PyComment{cosine similarity between pixel $i$ and $i^*$ for each $i$ in feature A}\\
    \PyCode{~~~~similarity = torch.nn.CosinSimilarity(ftA\_flat, ftA\_star\_flat)}  \\
    \PyCode{~~~~wt = torch.nn.softmax(similarity)} \PyComment{softmax} \\
    \PyCode{~~~~wt = wt.reshape()} \PyComment{unflatten}\\
    
    \PyCode{~~~~y = g\_ft\_A * wt} \\
    \PyCode{~~~~W\_y = W(y)} \PyComment{W is a $1\times 1\times 1$ torch.nn.Conv2d layer}\\
    \PyCode{~~~~z = ft\_A + W\_y} \\
    \PyFunc{~~~~return} \PyCode{z}
\caption{Pseudo code of Cycle-Resemblance Attention in PyTorch-like style.}
\label{algo:cra}
\end{algorithm*}

\noindent\textbf{Number of Attention Blocks.}
Additionally, to establish a more complementary sensitive analysis on the influence of the number of attention blocks, we conduct the experiment where the number of Cyc-Rsemblance blocks is set as $3$ on abdominal-MRI dataset under \textbf{\textit{setting 1}}.
All experimental results are shown in Table.~\ref{supblocks}, from which we can draw the same conclusion as we did in the main paper, where the optimal performance can be achieved when the number is set as $5$, and stacking multiple attention blocks has a beneficial effect on segmentation performance, while the excessive amount of blocks can also do harm to the model, making the network pay much attention on local details and thus ignore the global picture.

\noindent\textbf{Pseudo-code of Cycle-Resemblance Attention Module.} Our proposed cycle-resemblance attention module is shown in {Algorithm}~\ref{algo:cra}.

%说一下原因和结果
%main paper

% The number of blocks is increased from 1 to 9 with a step of 2.
